# Supplementary material for: BoDiffusion: Diffusing Sparse Observations for Full-Body Human Motion Synthesis
Source: arXiv:2304.11118 source file (2023-04-21)
Supplement: Supplementary file 1 [file figures_architecture_details.tex]

\begin{figure*}[t]
    \centering
    \includegraphics[width=0.82\linewidth]{fig/supplementary/simpleUnet.png}
    \caption{\textbf{\MODELNAME\ Architecture.} Our denoising model is based on U-Net architecture. We provide a detailed U-Net architecture for each block. 
    In particular, we denote the input and output dimensions of each block. 
    Besides, we provide further details in terms of structure on Figs.~\ref{fig:resblock}, \ref{fig:attention}, and \ref{fig:sampling}.
    Red dashed arrows represent down-sampling blocks with stride = 2, while blue dotted arrows represent up-sampling blocks with stride = 1/2.
    }
    \label{fig:unet}
    \vspace{20pt}
\end{figure*}

\begin{figure*}[t!]
    \centering
    \begin{subfigure}[t]{0.4\linewidth} 
        \includegraphics[width=1.0\linewidth]{fig/supplementary/rotRB.png}
        \caption{The timestep embedding is used in each residual block, where its linear projection is used to predict the scale and shift to transform intermediate activations. $\gamma_i$ defines the number of input and output channels for every convolutional layer, and $\zeta_i$ defines the projection dimensionality for the timestep embedding.}
        \label{fig:resblock}
    \end{subfigure}
    \hspace{0.07\linewidth}
        \begin{subfigure}[t]{0.2\linewidth} 
        \includegraphics[width=1.0\linewidth]{fig/supplementary/rotattentionblock.png}
        
        \caption{Structure of the single Attention Block in the middle of the U-Net. It consists of a GroupNorm~\cite{wu2018group}, two 1D convolutions, and an attention layer as in~\cite{Dhariwal2021DiffusionMB}.}
        \label{fig:attention}
    \end{subfigure}
    \hspace{0.05\linewidth}
        \begin{subfigure}[t]{0.2\linewidth} 
        \includegraphics[width=1.0\linewidth]{fig/supplementary/rotsampling.png}
        \caption{Number of input and output channels $k$ stays the same. Stride is $2$ for down-sampling and is $1/2$ for up-sampling.}
        \label{fig:sampling}
    \end{subfigure}
    \caption{\textbf{Detailed description of different blocks used in the U-Net model.}}
    \label{fig:blocks}
\end{figure*}
