# Supplementary material for: BoDiffusion: Diffusing Sparse Observations for Full-Body Human Motion Synthesis
Source: arXiv:2304.11118 source file (2023-04-21)
Supplement: Supplementary file 3 [file tab_sup_ablations.tex]

\begin{table*}[t!]
% \resizebox{\textwidth}{!}{%
\centering
\footnotesize
\begin{tabular}{lccccccccc@{}}
Name & $\#$ Params & MPJRE & MPJPE & MPJVE & Jitter & Hand PE & Hand RE & Pelvis PE & Pelvis RE \\ 
\toprule
% \MODELNAME\ (Input-cond) & 4.50 & 6.11 & 25.98 & 0.75 & 3.07 & 2.70 & 7.98 & 5.35\\
Predictive U-Net & 19M & 2.81 & 4.36 & 33.35 & 1.44 & 3.43 & 3.04 & 3.59 & 20.82 \\
\MODELNAME\ (Ours)  & 22M  & \textbf{2.48} & \textbf{3.62} & \textbf{20.65} & \textbf{1.24} & \textbf{2.91} & \textbf{2.70} & \textbf{3.11} & \textbf{4.79} \\
\bottomrule
\end{tabular}%
% } %resizebox
\caption{\textbf{Predictive model vs Generative model.} 
To fully demonstrate the effectiveness of the denoising power of our DDPM, we train a predictive model using the framework of~\cite{jiang2022avatarposer}. 
% That is, we train with a temporal window of 41 consecutive frames.
To make it comparable with \MODELNAME, we use our U-Net architecture instead of the transformer architecture~\cite{jiang2022avatarposer}. The slight difference in the number of parameters between these models is due to the reduced number of input channels in Predictive U-Net because it uses only conditioning signal $s^{1:W}, W=41$ as input.
% We demonstrate the importance of using the DDPM denoising protocol. 
Our model significantly outperforms the Predictive U-Net baseline in all the metrics.
We report MPJPE [cm], MPJRE [$\deg$], MPJVE [cm$/$s], and Jitter [km$/\text{s}^3$] on a subset of AMASS dataset (CMU, BMLrub, and HDM05).}
\label{tab:sup_ablations}
\end{table*}
