# Supplementary material for: BoDiffusion: Diffusing Sparse Observations for Full-Body Human Motion Synthesis
Source: arXiv:2304.11118 source file (2023-04-21)
Supplement: Supplementary file 4 [file tab_sup_ablations_ik.tex]

\begin{table*}[]
% \resizebox{\textwidth}{!}{%
\footnotesize
\centering

\begin{tabular}{lcccccccccc}
\multirow{2}{*}{Method} & \multicolumn{2}{c}{\textit{Inverse Kinematics}} & \multirow{2}{*}{MPJRE} & \multirow{2}{*}{MPJPE} & \multirow{2}{*}{MPJVE} & \multirow{2}{*}{Jitter} & \multirow{2}{*}{Hand PE} & \multirow{2}{*}{Hand RE}  & \multirow{2}{*}{Pelvis PE} & \multirow{2}{*}{Pelvis RE} \\
& \textit{LR}& \textit{Iters.} \\  % &  &  &  &  &  &  & & &  & &                                   
\toprule
\multirow{2}{*}{AvatarPoser~\cite{jiang2022avatarposer}}& \textemdash & \textemdash&2.92 & 3.95 & 26.80 & 1.42 & {2.10} & 2.96 & 3.24 & 19.69\\

 & $1e-2$&80&2.96&3.74&25.59&1.46&\textbf{0.12}&3.20&3.24&19.69 \\
 \midrule
 \multirow{2}{*}{\MODELNAME\ (Ours) }& \textemdash & \textemdash & 2.48 & {3.62} & {20.65} & {1.24} & 2.91 & \textbf{2.70} & \textbf{3.11} & {4.79}\\

 & $1e-2$  &   80  &2.59&\textbf{3.31}&\textbf{19.10}&\textbf{1.21}& \underline{0.13} &\textbf{2.70}&\textbf{3.11}& 4.81\\
\bottomrule
\end{tabular}
% }
\caption{\textbf{Inverse Kinematics (IK).} As a complementary experiment, we report the results with IK~\cite{jiang2022avatarposer} as post-processing for the hands.
We can see that using the IK module to refine the prediction results in an almost perfect alignment of hands with the GT tracking position for both Our method and AvatarPoser.
% Therefore,  
We report MPJPE [cm], MPJRE [$\deg$], MPJVE [cm$/$s], and Jitter [km$/\text{s}^3$] metrics.}
\label{tab:sup_ablations_IK}
\end{table*}
